# Supplementary material for: Overcoming Generic Knowledge Loss with Selective Parameter Update
Source: arXiv:2308.12462 source file (2024-04-19)
Supplement: Supplementary file 1 [file supp.tex]

\documentclass[10pt,onecolumn,letterpaper]{article}

\usepackage{cvpr}   
\usepackage[accsupp]{axessibility}
\input{24cvpr/preamble}

\definecolor{cvprblue}{rgb}{0.21,0.49,0.74}
\usepackage[pagebackref,breaklinks,colorlinks,citecolor=cvprblue]{hyperref}

\title{Overcoming Generic Knowledge Loss with Selective Parameter Update  Supplementary Materials}

\begin{document}
\maketitle
\tableofcontents
{
\input{content_paper/appendix}
    \small
    \bibliographystyle{ieeenat_fullname}
    \bibliography{reference}
}

\end{document}
